# Supplementary material for: LaMAR: Benchmarking Localization and Mapping for Augmented Reality
Source: arXiv:2210.10770 source file (2022-10-19)
Supplement: Supplementary file 1 [file trajectories_CAB.tex]

\def\iwidth{0.3295}
\def\hwidth{0.005}

\begin{minipage}{\iwidth\textwidth}
    \centering
    \includegraphics[width=\linewidth]{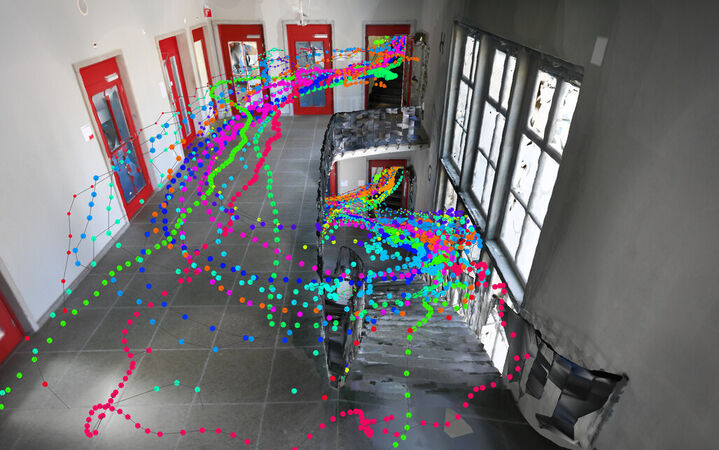}\\
    \includegraphics[width=\linewidth]{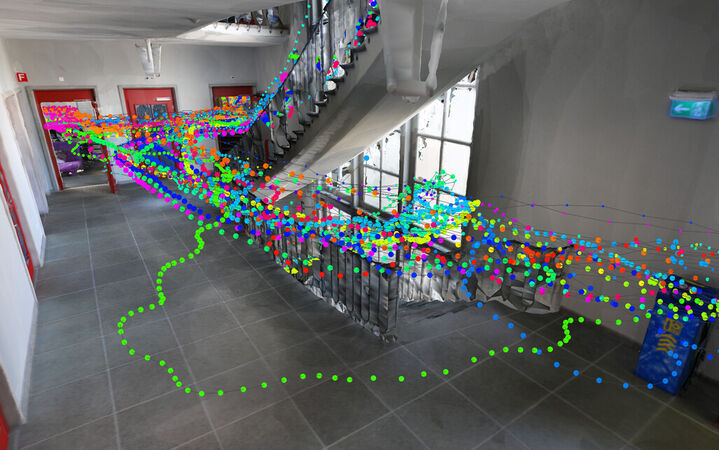}%
\end{minipage}%
\hspace{\hwidth\textwidth}%
\begin{minipage}{0.664\textwidth}
    \centering
    \includegraphics[width=\linewidth]{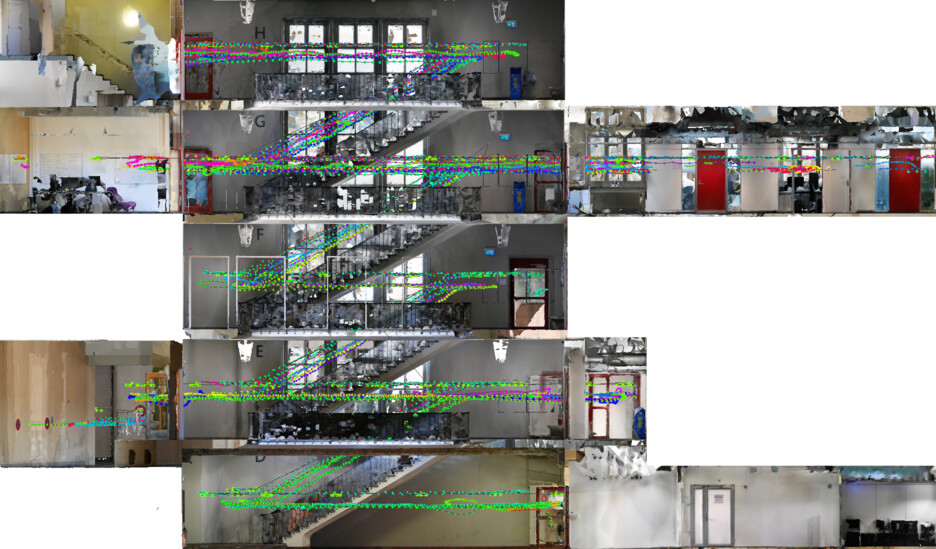}%
\end{minipage}%
\vspace{\hwidth\textwidth}

\includegraphics[width=\iwidth\linewidth]{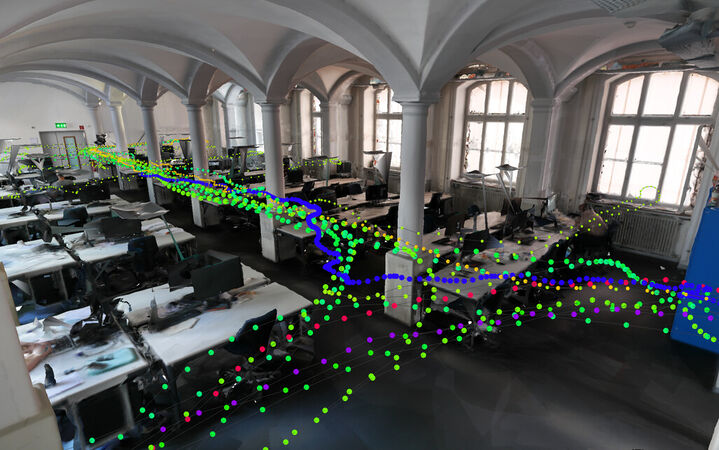}%
\hspace{\hwidth\textwidth}%
\includegraphics[width=\iwidth\linewidth]{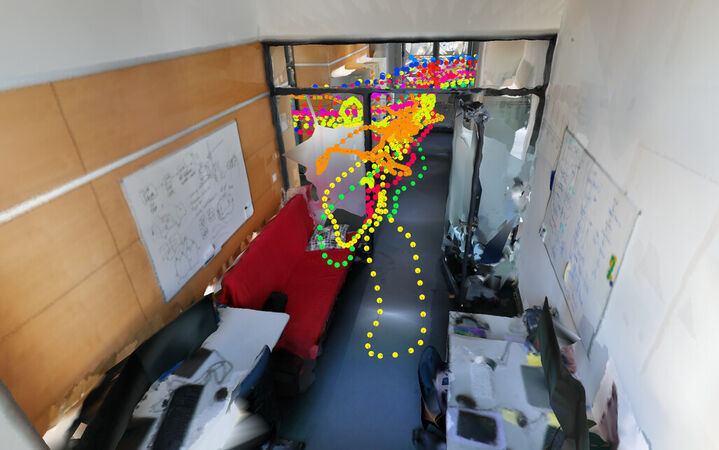}%
\hspace{\hwidth\textwidth}%
\includegraphics[width=\iwidth\linewidth]{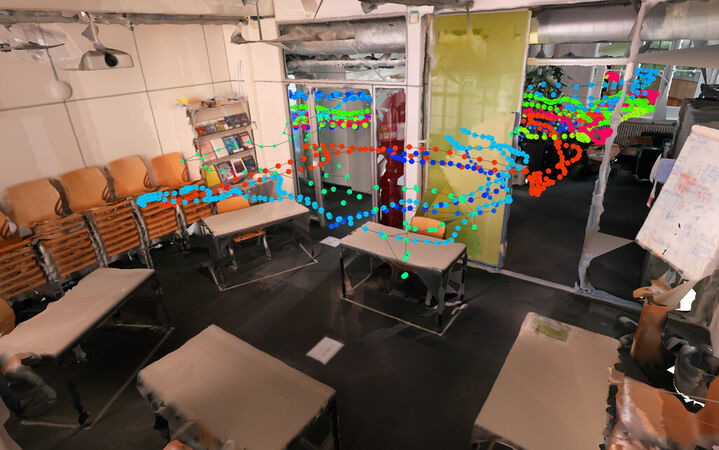}%
\vspace{\hwidth\textwidth}

\includegraphics[width=\iwidth\linewidth]{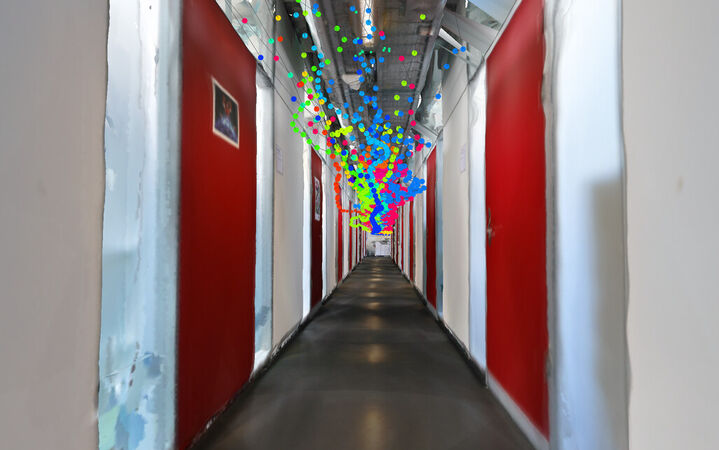}%
\hspace{\hwidth\textwidth}%
\includegraphics[width=\iwidth\linewidth]{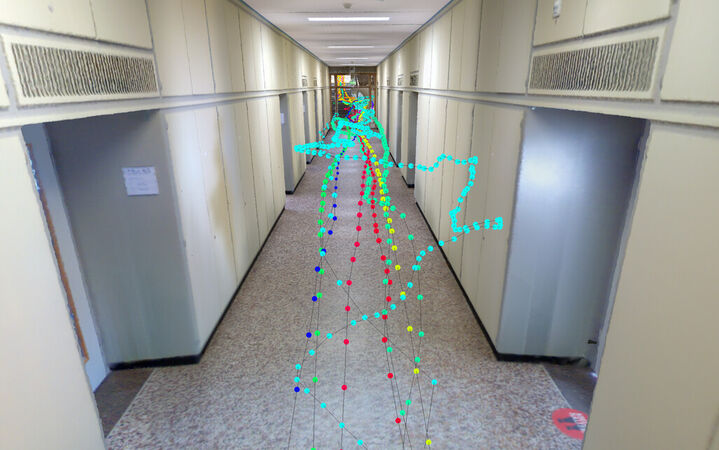}%
\hspace{\hwidth\textwidth}%
\includegraphics[width=\iwidth\linewidth]{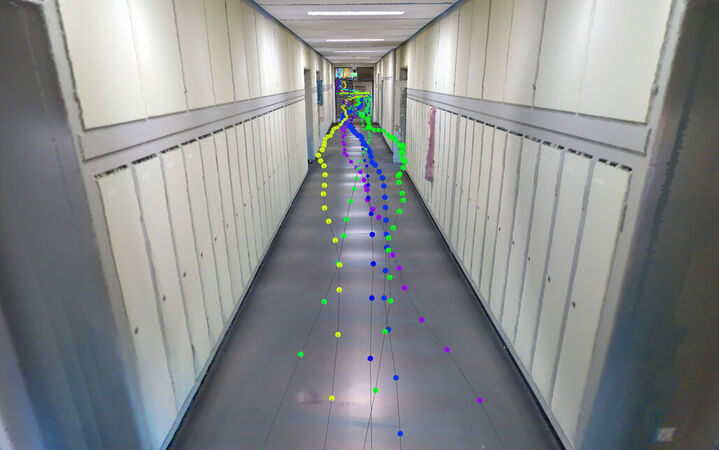}%
\vspace{\hwidth\textwidth}

\includegraphics[width=\iwidth\linewidth]{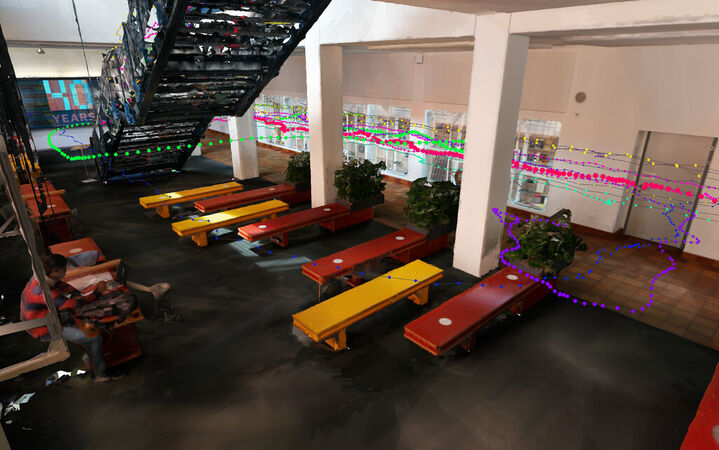}%
\hspace{\hwidth\textwidth}%
\includegraphics[width=\iwidth\linewidth]{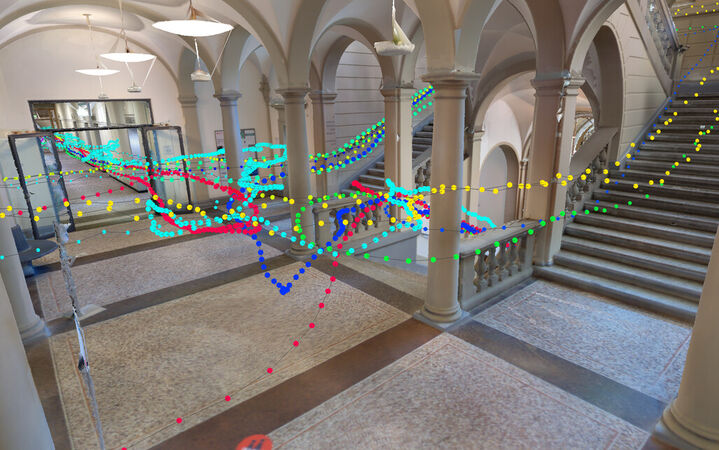}%
\hspace{\hwidth\textwidth}%
\includegraphics[width=\iwidth\linewidth]{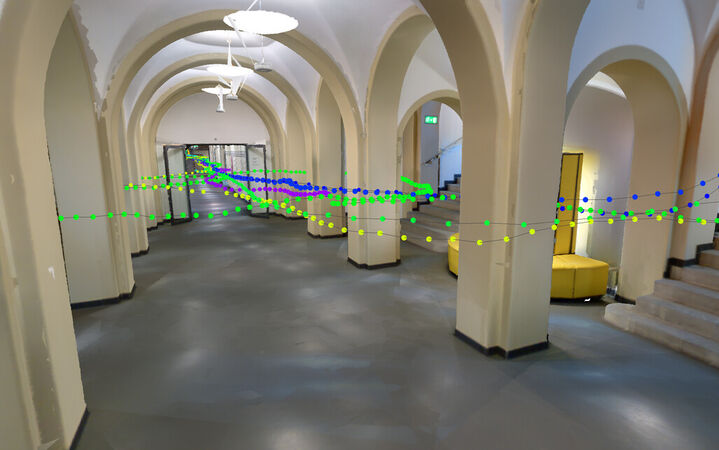}%
\vspace{\hwidth\textwidth}

\includegraphics[width=\iwidth\linewidth]{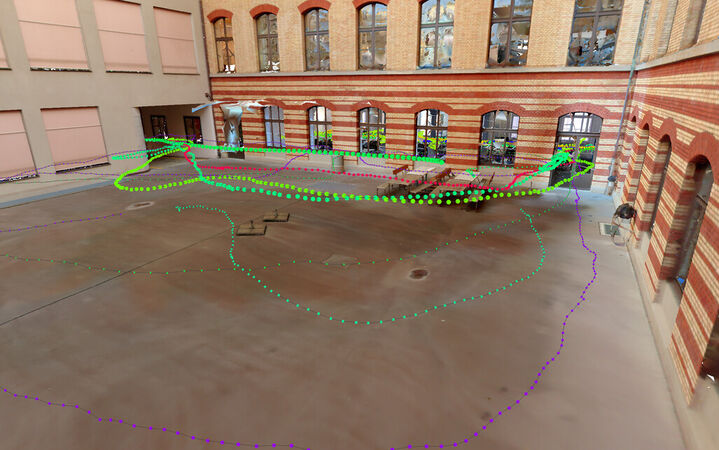}%
\hspace{\hwidth\textwidth}%
\includegraphics[width=\iwidth\linewidth]{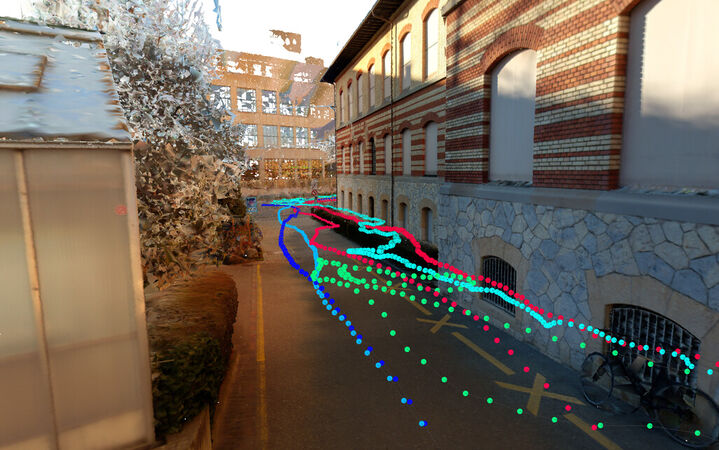}%
\hspace{\hwidth\textwidth}%
\includegraphics[width=\iwidth\linewidth]{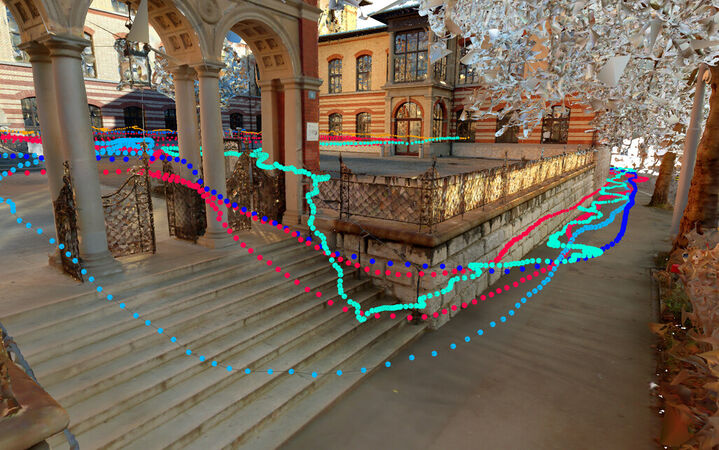}%
