# Supplementary material for: LaMAR: Benchmarking Localization and Mapping for Augmented Reality
Source: arXiv:2210.10770 source file (2022-10-19)
Supplement: Supplementary file 5 [file trajectories_LIN.tex]

\def\iwidth{0.3295}
\def\hwidth{0.005}

\includegraphics[width=\iwidth\textwidth]{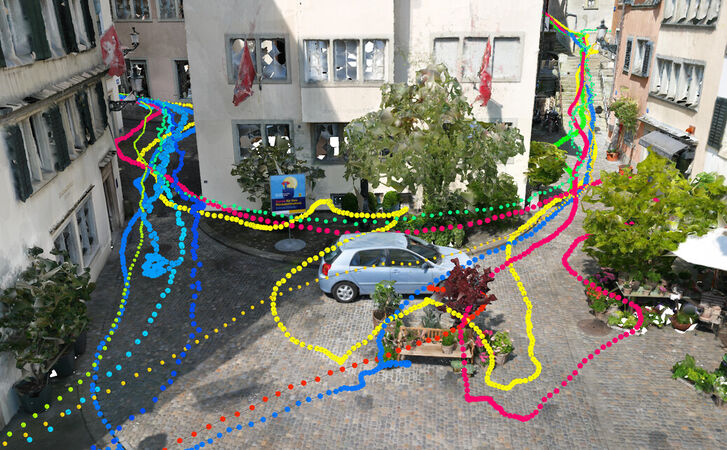}%
\hspace{\hwidth\textwidth}%
\includegraphics[width=\iwidth\textwidth]{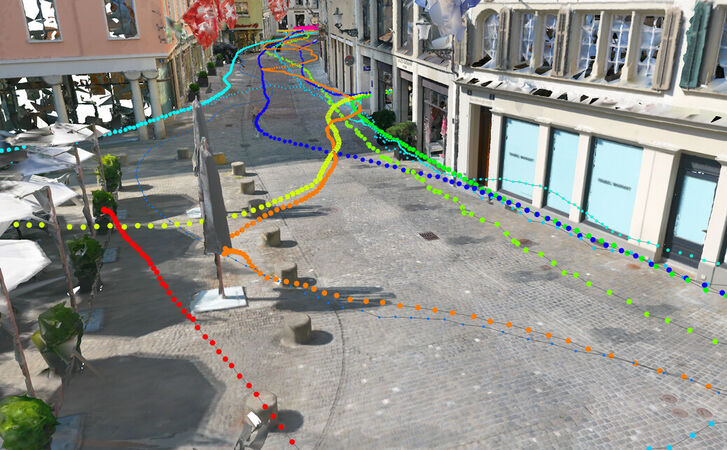}%
\hspace{\hwidth\textwidth}%
\includegraphics[width=\iwidth\textwidth]{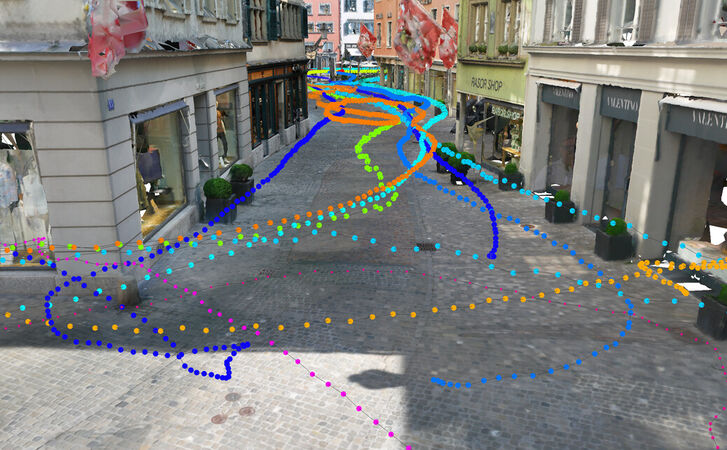}%
\vspace{\hwidth\textwidth}

\includegraphics[width=\iwidth\textwidth]{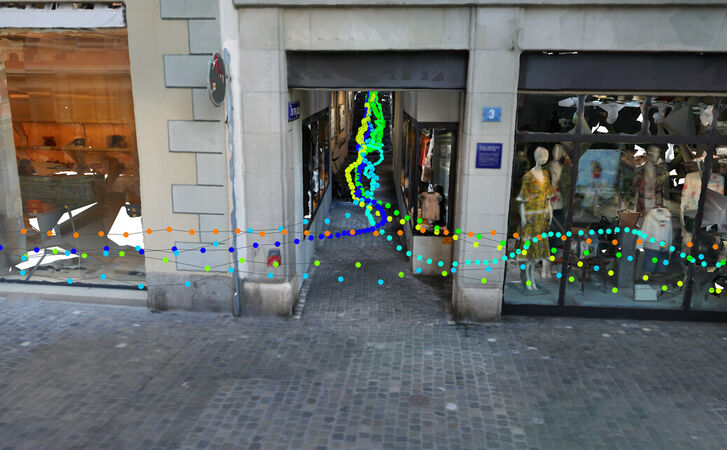}%
\hspace{\hwidth\textwidth}%
\includegraphics[width=\iwidth\textwidth]{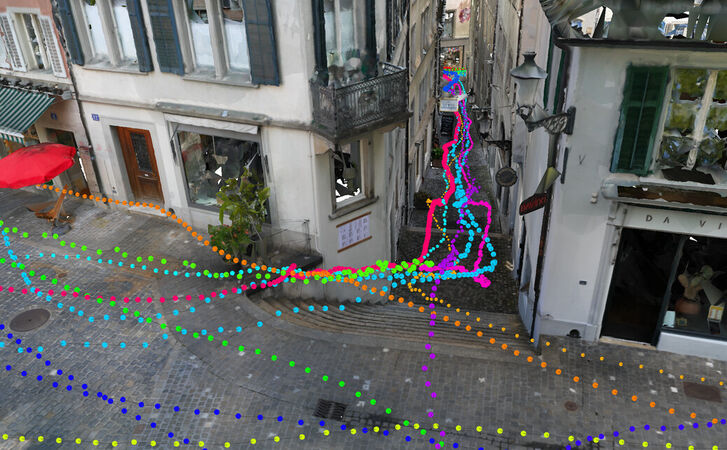}%
\hspace{\hwidth\textwidth}%
\includegraphics[width=\iwidth\textwidth]{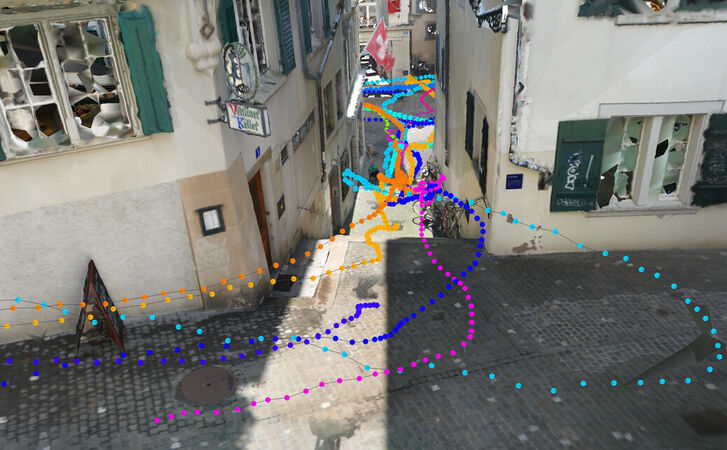}%
\vspace{\hwidth\textwidth}

\includegraphics[width=\iwidth\textwidth]{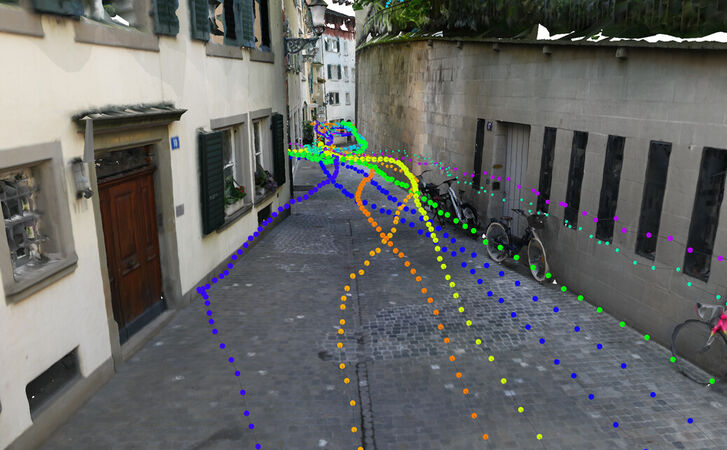}%
\hspace{\hwidth\textwidth}%
\includegraphics[width=\iwidth\textwidth]{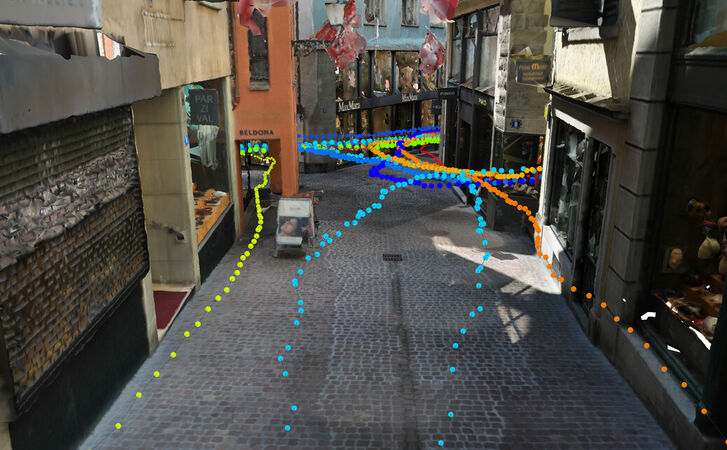}%
\hspace{\hwidth\textwidth}%
\includegraphics[width=\iwidth\textwidth]{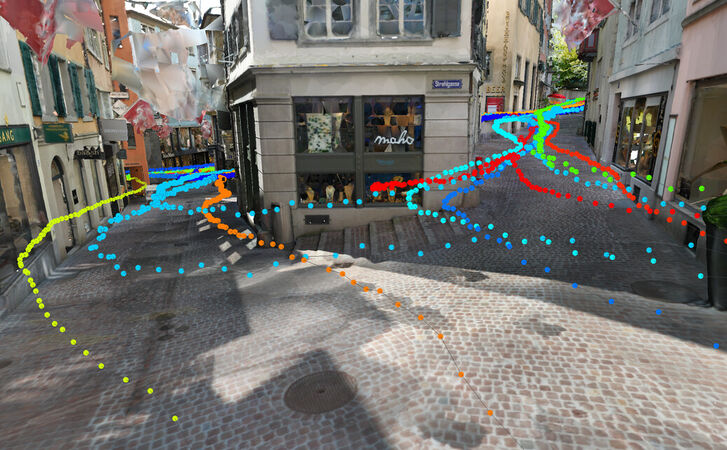}%
