# Supplementary material for: LaMAR: Benchmarking Localization and Mapping for Augmented Reality
Source: arXiv:2210.10770 source file (2022-10-19)
Supplement: Supplementary file 6 [file uncertainties.tex]

\def\iwidth{0.60}
\def\histwidth{0.389}
\def\hwidth{0.01}

\includegraphics[width=\iwidth\textwidth]{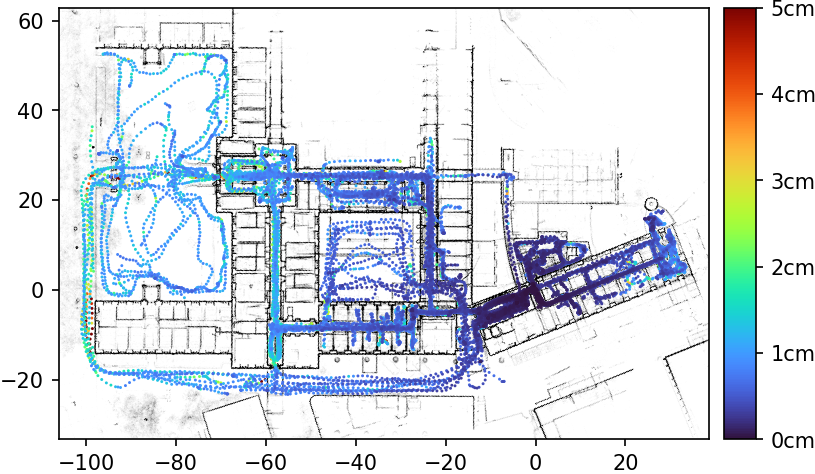}%
\hspace{\hwidth\textwidth}%
\includegraphics[width=\histwidth\textwidth]{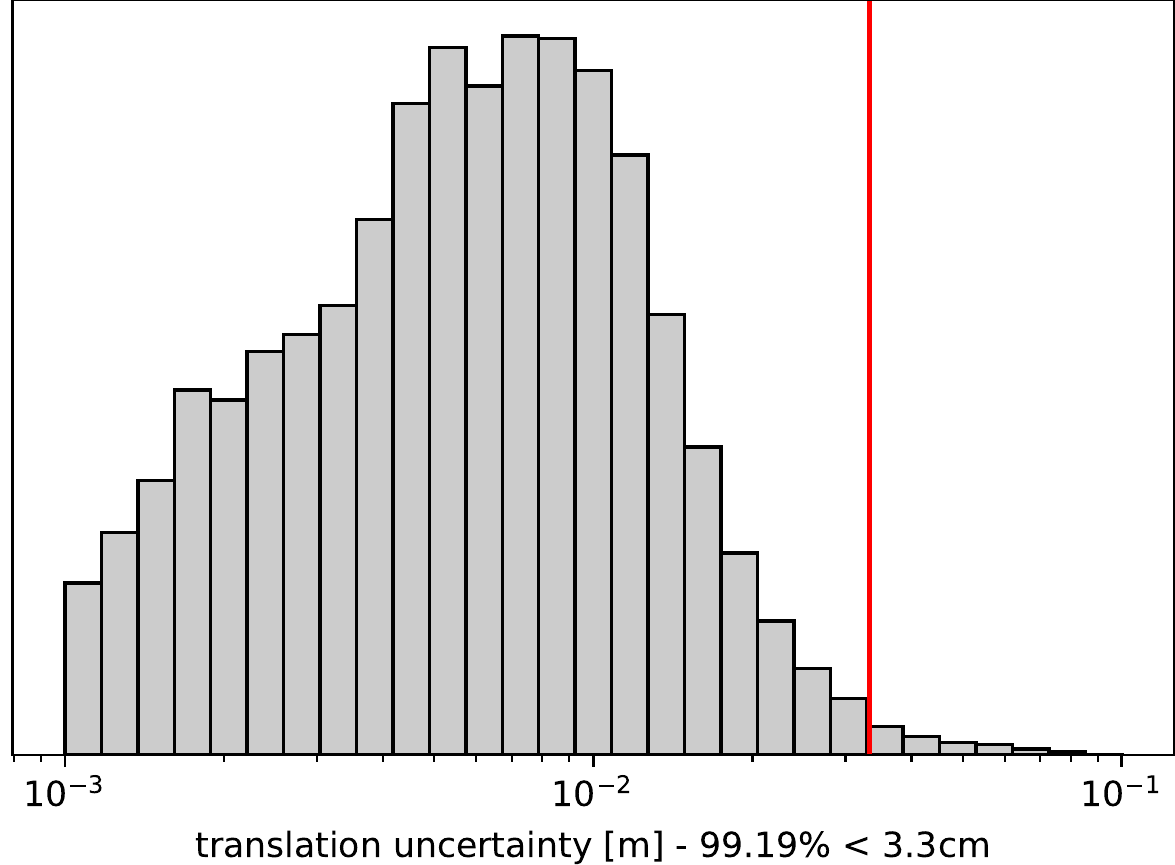}%
\vspace{4mm}

\includegraphics[width=\iwidth\textwidth]{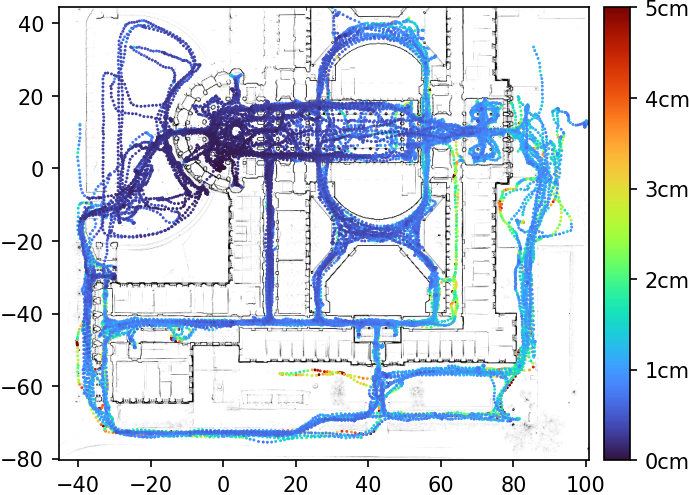}%
\hspace{\hwidth\textwidth}%
\includegraphics[width=\histwidth\textwidth]{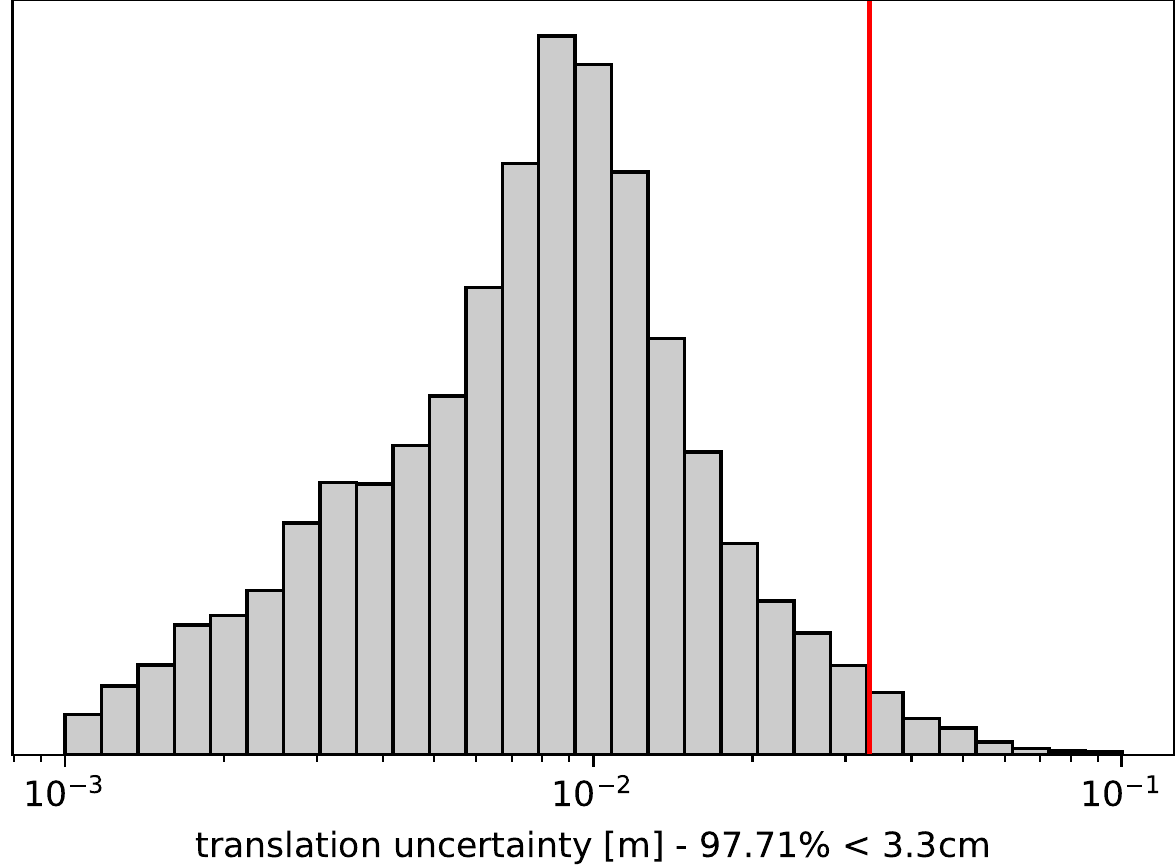}%
\vspace{4mm}

\includegraphics[width=\iwidth\textwidth]{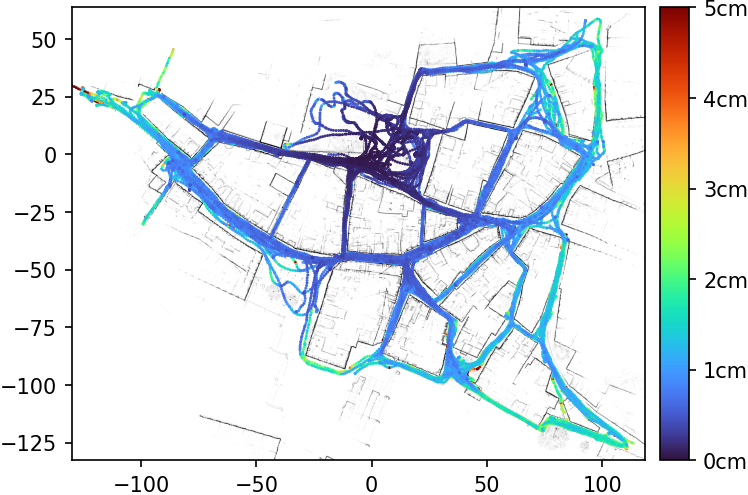}%
\hspace{\hwidth\textwidth}%
\includegraphics[width=\histwidth\textwidth]{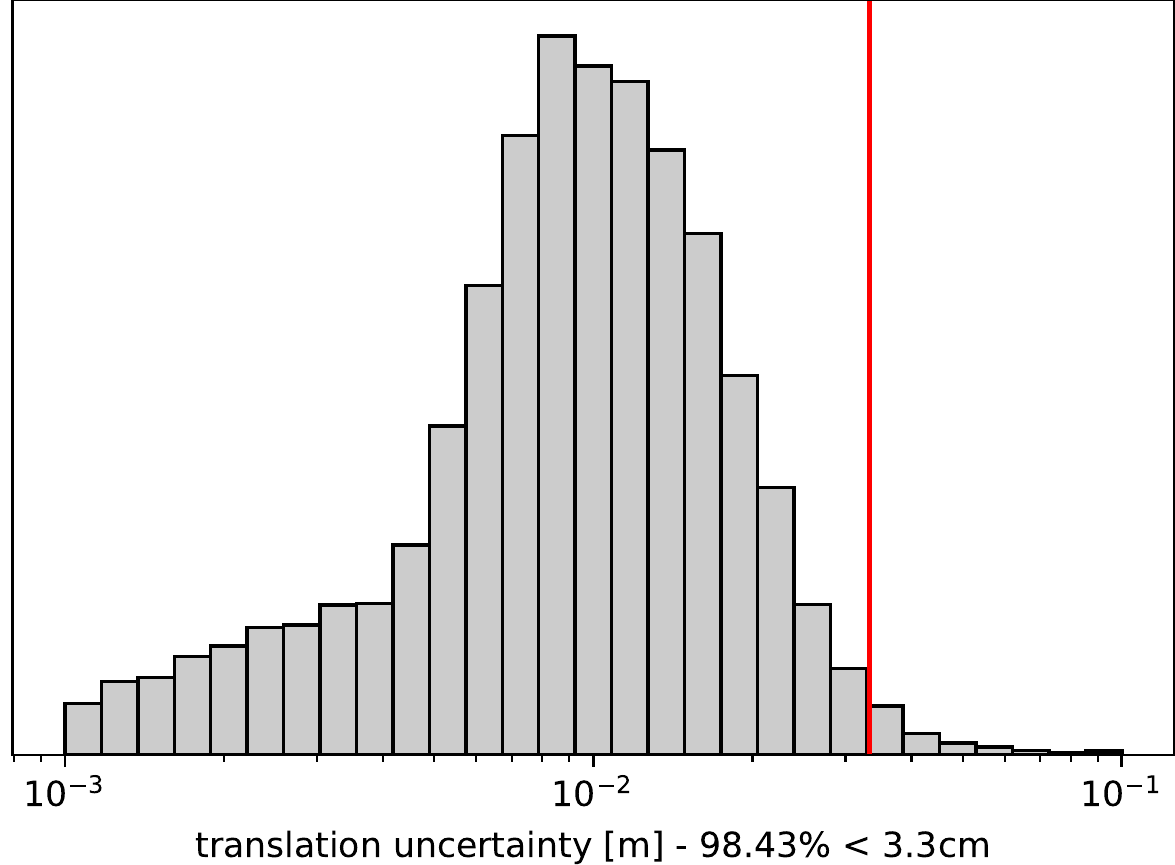}%
